# Supplementary material for: Impact Invariant Control with Applications to Bipedal Locomotion
Source: arXiv:2103.06907 source file (2021-10-01)
Supplement: Supplementary file 1 [file appendices.tex]

\section{Appendices}

\subsection{Derivation of No-Slip Rigid Body Reset Map}
\label{app:rigid_impact_model}

Using the instantaneous impact assumption and no-slip condition restated below:
\begin{align}
	M(v^+ - v^-) &= J^T \Lambda\\
	Jv^+ = 0
\end{align}
we can solve for the contact impulse $\Lambda$ and post-impact velocity $v^+$.
\begin{align}
	v^+ - v^- &= M^{-1} J^T \Lambda \nonumber\\
	Jv^+ - Jv^- &= J M^{-1} J^T \Lambda \nonumber\\
	\Lambda &= - (J M^{-1} J^T)^{-1} J v^-\\
	v^+ &= v^- - M^{-1} J^T (J M^{-1} J^T)^{-1} J v^- \nonumber\\
	v^+ &= (I - M^{-1} J^T (J M^{-1} J^T)^{-1} J) v^-
\end{align}

\subsection{Mapping Cost-to-go Across Impacts}
\label{app:hlqr_mapping}

Under the instantaneous impact assumption, the cost-to-go cannot change during the impact event, which results in the expression:
\begin{align}
\lim_{t \rightarrow t^-} \tilde{x}(t)^T S(t) \tilde{x}(t) &= \lim_{t \rightarrow t^+} \tilde{x}(t)^T S(t) \tilde{x}(t)
\end{align}
Using (\ref{eq:reset_map}), we can relate $\tilde{x}^-$ and $\tilde{x}^+$ with the linearized reset map $\hat{R}$:
\begin{align}
\lim_{t \rightarrow t^-} \tilde{x}(t) = \hat{R} \lim_{t \rightarrow t^+} \tilde{x}(t)
\end{align}
Through substitution, we arrive at the expression to map $S$ across an impact event.
\begin{align}
S(t^-) &= \hat{R}^T S(t^+) \hat{R}
\end{align}

\subsection{Finding Gaits using Trajectory Optimization}
\label{app:traj_opt}

The walking and jumping gaits were found through trajectory optimization by formulating them as constrained direct collocation problems and solving using a C++ implementation of DIRCON \cite{posa2016optimization}.
For both trajectories, I imposed no-slip contact constraints on the feet that were defined to be in stance as well as appropriate joint and actuator limits.
These can both be represented as the following optimization problem:
\begin{align}
	\min_{x_k, u_k}   &\quad&  \sum_{k} g(x_k, u_k) + g_f(x_N) &&  & \\
	\text{subject to: } 
	&\quad&  c(x, u) = 0 &&  & \\
	&\quad&  \phi(q) = \psi(x) = \alpha(x, u, \lambda) = 0 \\
	&\quad&  h(x, u) \geq 0  &&  &
\end{align}
\noindent where $g$ is a cost on the states and inputs, typically defined to be the $u^T u$ plus some normalization terms.
$c$ are the equality constraints such as the dynamics constraints at the collocation points and $h$ are the inequality constraints such as joint and actuator limits.
$\phi$ and its first and second time derivatives $\psi$ and $\alpha$ respectively are kinematic constraints.
These are the no-slip contact constraints and for Cassie specifically, the loop closure constraint between the thigh and the hip.

The walking trajectory was composed of two modes, with a single foot in stance per mode.
I set periodic constraints, which enforced that the final state must equal the initial state except for the global x position of the hip, which was instead constrained to translate 0.3m over the full trajectory.
I also set symmetry constraints between the left and right legs; note that setting symmetry constraints is equivalent to generating a trajectory for a single stance mode and simply mirroring the state to construct the trajectory for the second mode.
I chose to set symmetry constraints for the ease of not having to post-process the final trajectory.

The jumping trajectory consisted of three modes {CROUCH, FLIGHT, STANCE}.
All four points of contact of Cassie were constrained to be on the ground for both the CROUCH and STANCE modes.
To enforce a jumping motion, I set that the height of the pelvis must be 0.2 m above the initial starting height, which was set at 1.075m.
I also constrained the initial and final state to have zero initial velocity to prevent the optimizer from abusing initial kinematic energy in the system.
